# Supplementary material for: Learning Physical Models that Can Respect Conservation Laws
Source: arXiv:2302.11002 source file (2023-10-11)
Supplement: Supplementary file 1 [file app_detailed_proofs.tex]

\section{Detailed proofs} 
\label{app:convergence_to_operator}

\michael{This section I think needs to be completely re-organized.  Be more precise about what equation/lemma/theorem we are proving. Add more material to guide the reader on what we are doing, e.g. full rank vs. not.}

\subsection{Finite case}

\begin{lemma}
Consider the constraint matrix \(G\). The matrix \(A\) defined in \autoref{eq:physnp_posterior} has $A v = v$ for $v \in (\ker G)$. 
\end{lemma}

\paragraph{Proof.}
Consider $v \in (\ker G)$.
Then $Av = (I + \Sigma F^T \Sigma_F^{-1} F) v = v + \Sigma F^T \Sigma_F^{-1} F v = v$. \gaurav{what is F? should be G}

\begin{lemma}
$\|Av\| > \|v\|$ for $v \in (\ker G)^\perp$.
\end{lemma}

\paragraph{Proof.}
Consider $v \in (\ker G)^\perp$. 
Let $H \equiv \Sigma G^T \Sigma_G^{-1} G$.
Note that $H$ is positive semi-definite.
Then \(\|Av\|^2 = v^T v + 2 v^T G v + v^T G^T G v = \|v\|^2 + 2 v^T G v + v^T G^T G v \) \gaurav{fix typo, should be H here}. Since $Gv$ is non-zero, $\|Av\|^2 > \|v\|^2$ as required. \gaurav{you can claim $\geq$ due to 'semi-definite'.}

\subsection{Convergence to exact linear constraint}

\begin{lemma} \label{lemma:constraint_noise_to_zero}
Let $\Sigma_G^m = \sigma^2_m I$ define the covariance of the linear constraint. As $\sigma^2_m \to 0$,
$ G \tilde u_{m} - b \to 0$.
\end{lemma}

\paragraph{Proof.}
First, assume $b = 0$.
Let $\tau^2_m \equiv \frac{1}{\sigma^2_m}$. Then the associated $A_m$ is:
\[
A_m = (I + {\tau^2_{m}}\Sigma G^T G)
\]
Let $v_1, \dots, v_p$ be the eigenvectors of $A_m$ where $\lambda_i > 1$, and $v_{p+1} \dots v_{N}$ be the remaining eigenvectors with $\lambda = 1$.
If $\alpha_1, \dots, \alpha_p$ are the non-zero eigenvalues of $\Sigma G^T G$, then
\[
\lambda_i = (1 + \tau_m^2 \alpha_i)
\]
For $A_m^{-1}$, this implies the associated eigenvector is $\frac{1}{1 + \tau_k^2 \alpha_i}$.

$\tilde \mu_m = A_m^{-1} \mu = \sum_{i=1}^p \frac 1 {\lambda_i} v_i + \sum_{i=p+1}^N v_i$ \gaurav{not sure how you wrote this??}.
As $m \to \infty$, $\frac 1 \lambda_i \to 0$, so $\tilde \mu_m \to \sum_{i=p+1}^N v_i$. Then $G \tilde \mu_m \to \sum_{i=p+1}^N Gv_i = 0$, as required. \gaurav{why eig vect of $G$ and $\Sigma G^TG$ would be equal? did we mentioned that $\Sigma$ is diagonal?}
\subsection{Continuous case}

\paragraph{Setup.}

Let $\mathcal G: \mathcal U \to \mathcal S$ be a linear operator from two infinite-dimensional function spaces with domains in $\udomain$ and $\sdomain$, respectively.
Concretely, we suppose $\mathcal U$ and $\mathcal S$ are reproducible \gaurav{reproducing} kernel Hilbert spaces (RKHS) with kernels $K_U: \udomain \times \udomain \to \mathbb R$ and $K_{\mathcal S}: \sdomain \times \sdomain \to \mathbb R$.

For both $\mathcal U$ and $\mathcal S$, we construct a sequence of grids $\xgridj, \sgridk$ where $\xgridj \subset \xgridseq{j+1}$ and $\sgridk \subset \sgridseq{k+1}$ with the following properties: 

(A1) For any $x \in \udomain$, \gaurav{and a given finite $\delta$,} there exists a $j^\star$ and $x^\prime$ such that $x^\prime \in \xgridj$ for \gaurav{for all?} $j \ge j^\star$ and $\|x^\prime - x\|_2 < \delta$.

(A2) For any $x \in \sdomain$, there exists a $k^\star$ and $x^\prime$ such that $x^\prime \in \sgridk$ for $k \ge k^\star$ and $\|x^\prime - x\|_2 < \delta$.
\danielle{Add additional sentence on uniform in kernel $y$ direction and in kernel $x$ direction}

%\danielle{relation to $N_j$ and $N_k \rightarrow \infty$}
%such that $\xgridj = [x_{U, 1}, \dots, x_{U, N_j}]$ for $x_{U, i} \in \mathcal X$ and $\sgridk = [x_{S, 1}, \dots, x_{S, N_k}]$ for $x_i \in \mathcal X_S$.

Let $\Phi_{U, j}: \mathcal U \to \mathbb R^{N_j}$ be the evaluation operator on $\mathcal U$ applied to the grid $\xgridj$ ( i.e., $\Phi_{U, j} u = [u(x_{U, i}]_{i = 1, \dots, N_j}$). This can be represented with $K_U$ by $\Phi_{U, j} u = [ \langle K_U(x_{U, i}, \cdot), u \rangle ]_{i = 1, \dots, N_j}$.
The adjoint of $\Phi_{U, j}$ is written $\Phi_{U, j}^T : \mathbb R^{N_j} \to \mathcal U$, where $\Phi_{U, j}^T a = \sum_{i=1}^{N_j} a_i K_U (x_{U, i}, \cdot)$ for $a \in \mathbb R^{N_j}$. \gaurav{is this defn of adjoint correct? can you provide some references here.}
We define an analogous sequence of operators $\Phi_{S, k}: \mathcal S \to \mathbb R^{N_k}$. 

For notation, let $\xgridprojj \equiv \Phi_{U, j}^T (\Phi_{U, j} \Phi_{U, j}^T)^{-1} \Phi_{U, j}$ and $\sgridprojk \equiv \Phi_{S, k}^T (\Phi_{S, k} \Phi_{S, k}^T)^{-1} \Phi_{S, k}$ represent the projections

\begin{lemma}
As $j \to \infty$ and $k \to \infty$, \ for any $u \in \mathcal U$ and $b \in \mathcal S$,

\begin{enumerate}
    \item $\xgridprojj u \to u$.
    \item $\sgridprojk b \to b$.
\end{enumerate}
\end{lemma}
This provides that as we increase the number of grid points in the function domain $\mathcal U$, our approximation will converge to the true function in the metric of $\mathcal U$.

\paragraph{Proof.}
The proofs for (1) and (2) are identical, so we will prove just (1).
Define $\phi_x \equiv K_{\mathcal U} (x, \cdot)$.
For a given $x \in \udomain$ and any $\epsilon > 0$, we can pick $\delta > 0$ such that, for any $x^\prime$ where $\|x - x^\prime\| < \delta$,
\begin{enumerate}
    \item $| u(x) - u(x^\prime)| < \epsilon / 2$
    \item $\| \phi_x - \phi_{x^\prime} \|_{\mathcal U} < \frac \epsilon {2 \| u\|_\mathcal{U}}$
\end{enumerate}
\gaurav{Given any x and $\delta$ why the above two would hold for $u(x)$?}
Now, using (A1), there is a $j^\star$ and $x^\prime$ such that $\| x - x^\prime \|_2 < \delta$ and $x^\prime \in \xgridj$.
For $x^\prime$ and $j \ge j^\star$ the following is true:
\[
\begin{split}
(\xgridprojj u) (x^\prime) &= \phi_{x^\prime}^T \xgridprojj u \\
&= e_{x^\prime}^T \Phi_{U, j} \Phi_{U, j}^T (\Phi_{U, j} \Phi_{U, j}^T)^{-1} \Phi_{U, j} u \\
&= e_{x^\prime}^T \Phi_{U, j}u \\
&= \phi_{x^\prime}^T u  = u(x^\prime)
\end{split}
\]
\gaurav{Do we need the above steps? Isn't this is implied from the defn that evaluations at the grid points are exact?}
Next, we bound the absolute difference between the projected $u$ evaluated at $x$ and $x^\prime$. This comes from the Cauchy-Schwartz inequality and the fact that a projection is a bounded operator.
\[
\begin{split}
|\phi_x^T \xgridprojj u - \phi_{x^\prime}^T \xgridprojj u| &= |\langle \phi_x - \phi_{x^\prime}, \xgridprojj u \rangle_{\mathcal U}| \\
&\le \|\phi_x - \phi_{x^\prime}\|_{\mathcal U} \|\xgridprojj u \|_{\mathcal U} \\
&\le  \|\phi_x - \phi_{x^\prime}\|_{\mathcal U} \|u\|_{\mathcal U} \\
& < \frac \epsilon 2
\end{split}
\]
Then it follows that $|\xgridprojj u (x) - u(x)| \le |\xgridprojj u (x) - \xgridprojj u(x^\prime)| + |u(x) - u(x^\prime)| < \epsilon$, proving (1).
% (A3) The evaluation operator on a simple point is uniformly bounded; i.e., $|b(x)| \le M_S \|b\|$ for finite $M$.

\begin{lemma} \label{lemma:seq_of_matrices}
There exists a sequence of matrices $G_{j, k}$ such that:
\begin{enumerate}
    \item $\Phi_{S, k}^T (\Phi_{S, k} \Phi_{S, k}^T)^{-1} G_{j, k} \Phi_{U, j} u \to \mathcal G u$. \danielle{consistency}
    \item $ \| G_{j, k} \Phi_{U, j} u - \Phi_{S, k} \mathcal G u \|_2 \to 0$
\end{enumerate}
as $j \to \infty$ and $k \to \infty$.

\end{lemma}

\paragraph{Proof.} 
We define $G_{j, k}$ as the following:
\[
G_{j, k} = \Phi_{S, k} \mathcal G \Phi_{U, k} (\Phi_{U, k} \Phi_{U, k}^T)^{-1}
\]
\gaurav{missing a transpose?}
\gaurav{$\mathcal{G}$ is from $\mathcal{U}\rightarrow\mathcal{S}$, so I am not sure what is $G_{j,k}$, is it like projection of the operator $\mathcal{G}$?}
Then,
\[
\Phi_{S, k}^T (\Phi_{S, k} \Phi_{S, k}^T)^{-1} G_{j, k} \Phi_{U, k} u = (\Phi_{S, k}^T (\Phi_{S, k} \Phi_{S, k}^T)^{-1} \Phi_{S, k}) \mathcal G (\Phi_{U, k} (\Phi_{U, k} \Phi_{U, k}^T)^{-1} \Phi_{U, k}) u
\]

From (A1) \gaurav{you mean from Lemma-4?}, $(\Phi_{U, j} (\Phi_{U, j} \Phi_{U, j}^T)^{-1} \Phi_{U, j}) u \to u$ as $j \to \infty$ and from (A2), $(\Phi_{S, k}^T (\Phi_{S, k} \Phi_{S, k}^T)^{-1} \Phi_{S, k}) \mathcal G u \to \mathcal G u$ as $k \to \infty$. Combining these two convergences leads to the desired result in (1).

For (2):
\[
\begin{split}
    \lim_{j \to \infty} \| G_{j, k} \Phi_{U, j} u - \Phi_{S, k} \mathcal G u \|_2 &= \lim_{j \to \infty}\|\Phi_{S, k} \mathcal G \Phi_{U, j} (\Phi_{U, j} \Phi_{U, j}^T)^{-1}  \Phi_{U, j} u - \Phi_{S, k} \mathcal G u \|_2 \\
    &= \|\Phi_{S, k} \mathcal G u - \Phi_{S, k} \mathcal G u \|_2 \\
    &= 0
\end{split}
% \|G_{j, k} \Phi_{U, j} u - \Phi_{S, k}  \mathcal G u\| = \|\Phi_{S, k} (\Phi_{S, k}^T (\Phi_{S, k} \Phi_{S, k}^T)^{-1} G_k \Phi_{U, k} u - \mathcal G u)\| \le M \|(\Phi_{S, k}^T (\Phi_{S, k} \Phi_{S, k}^T)^{-1} G_k \Phi_{U, k} u - \mathcal G u)\|_S \to 0
\]

\gaurav{I would suggest a complete re-write of this lemma. Lets declare $G_{j,k}$ as the projection of the operator $\mathcal{G}$ such that $G_{j,k} = \mathcal{P}_{S,k}\mathcal{G}\mathcal{P}_{U,j}$. This way the matrix $G$ has some meaning to it (projection/discretization of the operator). Then the lemma statement would be:
\\
The projection of the operator $\mathcal{G}$ is $G_{j,k}$ such that \\
$G_{j,k}\mathcal{P}_{U,j}u\rightarrow \mathcal{G}u$ as $j,k\rightarrow\infty$\\
I don't think we need the statement (2) of the lemma as it is pretty straightforward to deduce, but if we do wish to keep it, because we might be using the exact statement somewhere, then, lets reformulate as:\\
$\vert\vert G_{j,k}\mathcal{P}_{U,j}u - \mathcal{P}_{S,k}\mathcal{G}u\vert\vert_2\rightarrow 0$}

(A3) The constraint covariance matrix 

\begin{lemma}
We have the following: \gaurav{Needs to be restated in a proper way, refer $\tilde\mu_{j, k, m}$ to a proper definition location} \gaurav{You wish to claim point convergence or in L2?}
\[
\lim_{j \to \infty} \lim_{m \to \infty} G_{j, k} \tilde \mu_{j, k, m} - G_{j, k} \Phi_{U, j} u = 0
\]
\end{lemma}

\paragraph{Proof.}

Let $b_k \equiv \Phi_{S, k} \mathcal G u$ be the grid approximation of the constraint function $\mathcal G u$.
First, with Lemma \ref{lemma:seq_of_matrices} part (2),% we can find a $j^\prime$ such that $\| G_{j, k} u_k - b_k \|_2 < \epsilon$ for $j > j^\prime$.
\[
\lim_{j \to \infty}\| G_{j, k} \Phi_{U, j} u - b_k \|_2 = 0.
\]
Then, with Lemma \ref{lemma:constraint_noise_to_zero},% we can find an $m^\prime$ such that $\|G_k \tilde \mu_{k, m} - b_k \| < \epsilon$ for $m > m^\prime$.
\[
\lim_{m \to \infty}\| G_{j, k} \tilde \mu_{j, k,  m} - b_k \|_2 = 0.
\]
Combining these two limits gives the desired result.

% \begin{lemma}
% Define $\tilde \mu_k \equiv \lim_{m \to \infty} \mu_{k, m}$.
% \[
% \mathcal G P_k^{U \star} \tilde \mu_{k} \to \mathcal G u
% \]
% as $k \to \infty$.
% \end{lemma}
%\constraintconvergence*

\paragraph{Proof.}

We use multiple limits and add them together to get the desired result.
\[
\begin{split}
\mathcal G P_k^{U \star} \tilde \mu_{k} - P_k^{S \star} G_k \tilde \mu_{k} = \mathcal G P_k^{U \star} \tilde \mu_k - P_k^{S \star} G_k P_k^U P_k^{U \star} \tilde \mu_k &\to 0\\
P_k^{S \star} G_k \tilde \mu_{k} - P_k^{S \star} G_k P_k^U u &\to 0 \\
P_k^{S \star} G_k P_k^U u - \mathcal G u &\to 0
\end{split}
\]
With one additional assumption, we can show that \physnp converges to the exact solution for a fully defined linear system of PDES.

(Bijectivity) An inverse linear operator $\mathcal G^{-1}$ exists such that $\mathcal G^{-1} \circ \mathcal G$ is the identity map.

Then, by continuity,
$P_k^{U\star} \tilde \mu_k = \mathcal G^{-1} \mathcal G P_k^{U\star} \tilde \mu_k \to \mathcal G^{-1} \mathcal G u = u$, as required.
